# Supplementary material for: N-ACT: An Interpretable Deep Learning Model for Automatic Cell Type and Salient Gene Identification
Source: arXiv:2206.04047 source file (2022-05-08)
Supplement: Supplementary file 1 [file appendix.tex]

% \begin{thebibliography}{1}
%       \bibitem{scanpy}{
%  	abstract = {Scanpy is a scalable toolkit for analyzing single-cell gene expression data. It includes methods for preprocessing, visualization, clustering, pseudotime and trajectory inference, differential expression testing, and simulation of gene regulatory networks. Its Python-based implementation efficiently deals with data sets of more than one million cells (https://github.com/theislab/Scanpy). Along with Scanpy, we present AnnData, a generic class for handling annotated data matrices (https://github.com/theislab/anndata).},
%  	author = {Wolf, F. Alexander and Angerer, Philipp and Theis, Fabian J.},
%  	date = {2018/02/06},
%  	date-added = {2022-04-29 15:35:42 -0700},
%  	date-modified = {2022-04-29 15:35:48 -0700},
%  	doi = {10.1186/s13059-017-1382-0},
%  	id = {Wolf2018},
%  	isbn = {1474-760X},
%  	journal = {Genome Biology},
%  	number = {1},
%  	pages = {15},
%  	title = {SCANPY: large-scale single-cell gene expression data analysis},
%  	url = {https://doi.org/10.1186/s13059-017-1382-0},
%  	volume = {19},
%  	year = {2018},
%  	bdsk-url-1 = {https://doi.org/10.1186/s13059-017-1382-0},
%  }
%     \end{thebibliography}
% \begin{biblist*}[\normalsize]*{prefix={S\#}}
% \bib{scanpy}{article}{
% 	abstract = {Scanpy is a scalable toolkit for analyzing single-cell gene expression data. It includes methods for preprocessing, visualization, clustering, pseudotime and trajectory inference, differential expression testing, and simulation of gene regulatory networks. Its Python-based implementation efficiently deals with data sets of more than one million cells (https://github.com/theislab/Scanpy). Along with Scanpy, we present AnnData, a generic class for handling annotated data matrices (https://github.com/theislab/anndata).},
% 	author = {Wolf, F. Alexander and Angerer, Philipp and Theis, Fabian J.},
% 	date = {2018/02/06},
% 	date-added = {2022-04-29 15:35:42 -0700},
% 	date-modified = {2022-04-29 15:35:48 -0700},
% 	doi = {10.1186/s13059-017-1382-0},
% 	id = {Wolf2018},
% 	isbn = {1474-760X},
% 	journal = {Genome Biology},
% 	number = {1},
% 	pages = {15},
% 	title = {SCANPY: large-scale single-cell gene expression data analysis},
% 	url = {https://doi.org/10.1186/s13059-017-1382-0},
% 	volume = {19},
% 	year = {2018},
% 	bdsk-url-1 = {https://doi.org/10.1186/s13059-017-1382-0},
% }

% \end{biblist*}




% \bibliographystyle{StyleFiles/icml2022}
